# Supplementary material for: The Influence of the Java Collection Framework on Overall Energy Consumption
Source: arXiv:1602.00984 source file (2016-02-02)

# APPENDIX

Pereira, Couto, Cunha, Fernandes, and Saraiva

# Appendices

## A Set data for 25k population

| Methods | ConcurrentSkipListSet J | ms | HashSet J | ms | LinkedHashSet J | ms | TreeSet J | ms |
|---|---|---|---|---|---|---|---|---|
| add | 1.6822 | 87 | 1.7749 | 87 | 1.4917 | 75 | 1.4817 | 92 |
| addAll | 1.4549 | 93 | 1.4771 | 89 | 1.9335 | 94 | 1.5101 | 93 |
| clear | 1.4901 | 78 | 1.0586 | 64 | 1.3288 | 60 | 1.8566 | 73 |
| contains | 1.4213 | 88 | 2.0685 | 78 | 1.0401 | 76 | 2.0446 | 79 |
| containsAll | 1.8317 | 96 | 1.4000 | 77 | 2.1748 | 88 | 1.4443 | 89 |
| iterateAll | 1.9225 | 99 | 1.4554 | 92 | 1.2907 | 83 | 1.3844 | 83 |
| iterator | 1.6096 | 83 | 1.7596 | 75 | 0.9613 | 76 | 1.7239 | 76 |
| remove | 1.7877 | 78 | 1.2633 | 75 | 1.2458 | 93 | 1.0700 | 76 |
| removeAll | 1.8072 | 85 | 2.1359 | 77 | 1.9145 | 100 | 1.3920 | 91 |
| retainAll | 3.2607 | 206 | 2.4092 | 200 | 2.2512 | 199 | 3.2222 | 193 |
| toArray | 1.4789 | 86 | 1.3833 | 80 | 1.3776 | 79 | 1.6292 | 80 |

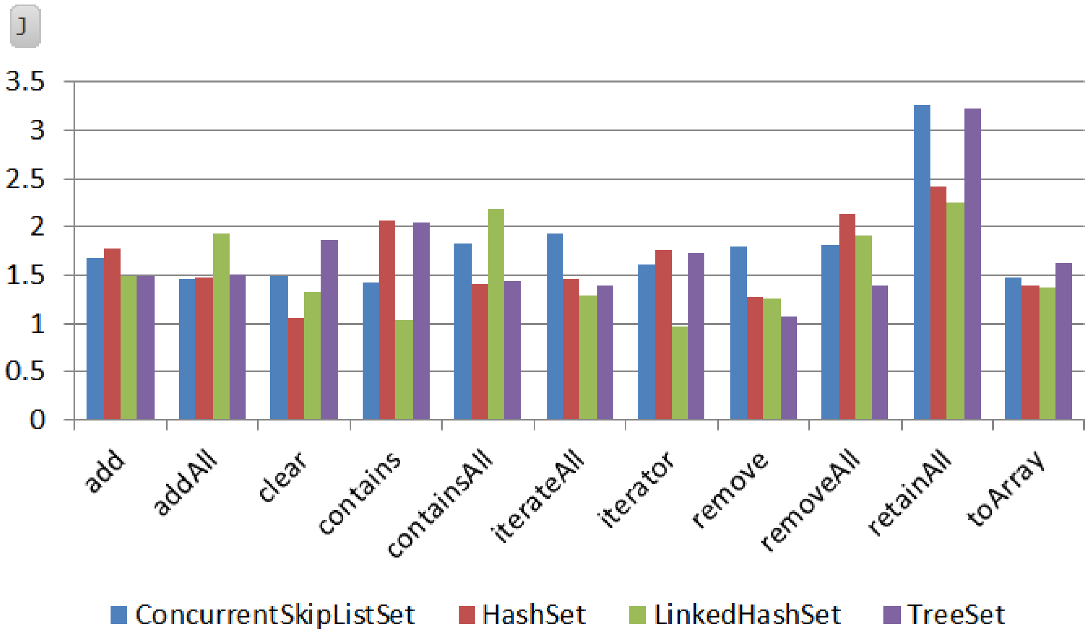

## B Set data for 250k population

| Methods | Concurrent SkipListSet J | ms | HashSet J | ms | Linked HashSet J | ms | TreeSet J | ms |
|---|---|---|---|---|---|---|---|---|
| add | 5.1254 | 284 | 5.5141 | 305 | 5.2348 | 277 | 4.2959 | 233 |
| addAll | 6.3474 | 391 | 5.5436 | 307 | 5.0125 | 279 | 4.5978 | 288 |
| clear | 4.2285 | 246 | 4.1085 | 227 | 4.6213 | 241 | 4.2033 | 229 |
| contains | 5.0685 | 272 | 5.2959 | 290 | 6.0423 | 251 | 4.5884 | 216 |
| containsAll | 6.5672 | 351 | 5.5917 | 291 | 5.1875 | 259 | 4.4657 | 254 |
| iterateAll | 5.4969 | 266 | 6.2567 | 298 | 5.3597 | 270 | 4.3067 | 247 |
| iterator | 4.9175 | 249 | 5.4548 | 290 | 5.1849 | 265 | 4.1703 | 214 |
| remove | 5.0868 | 260 | 5.3462 | 270 | 4.8186 | 255 | 4.2111 | 225 |
| removeAll | 5.7957 | 364 | 4.9622 | 295 | 5.2345 | 260 | 4.7445 | 278 |
| retainAll | 184.7828 | 17079 | 186.6178 | 17367 | 179.7946 | 16563 | 188.2510 | 17516 |
| toArray | 5.3265 | 270 | 5.7374 | 305 | 4.7959 | 271 | 4.5845 | 245 |

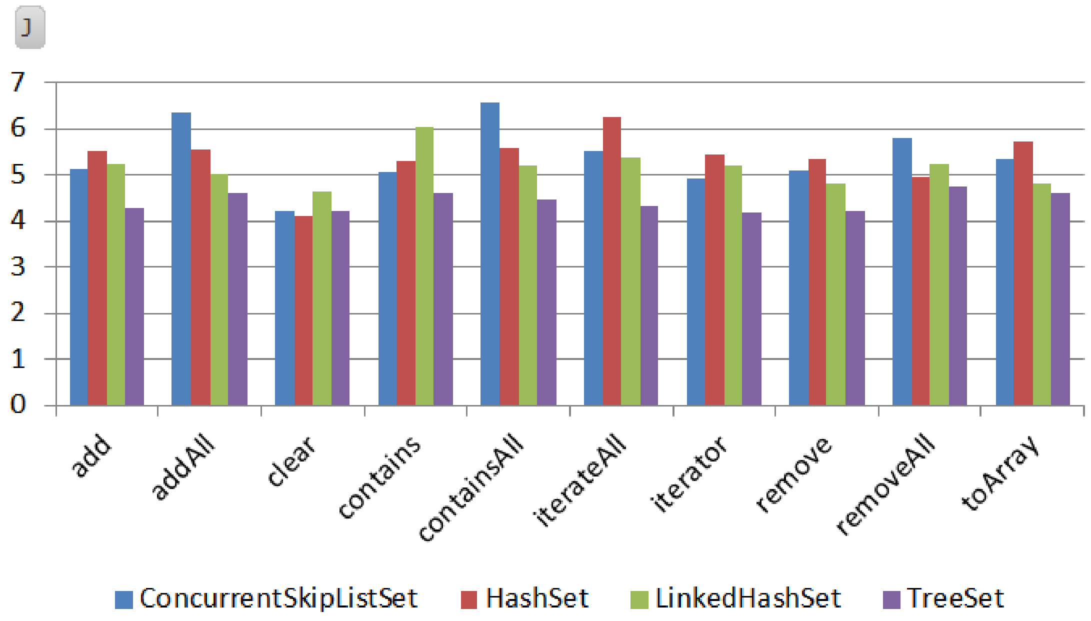

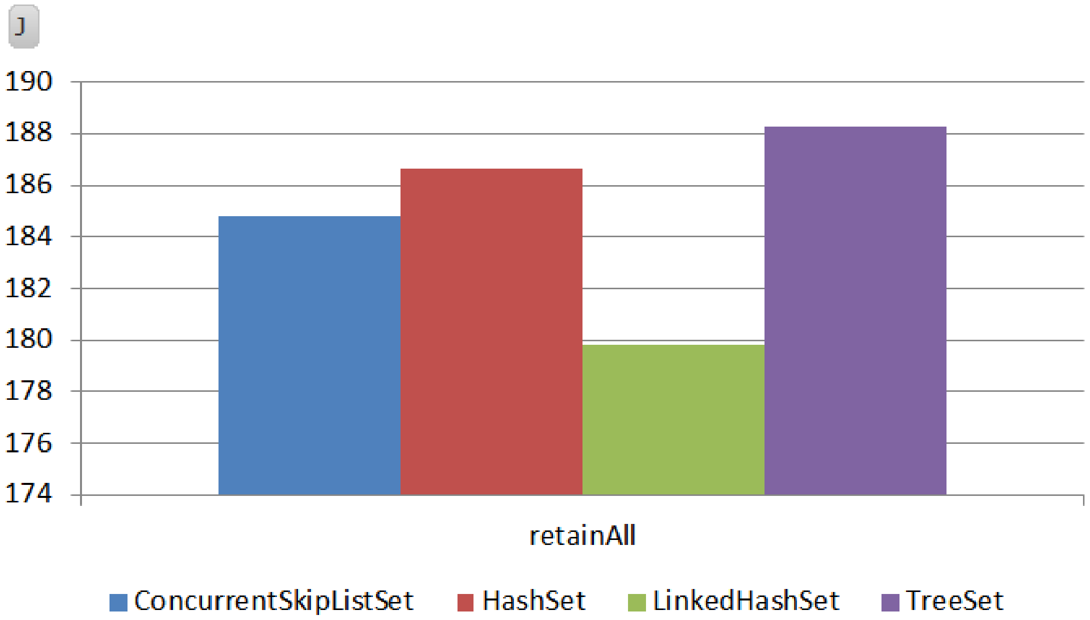
J
190
188
186
184
182
180
178
176
174
retainAll
ConcurrentSkipListSet
HashSet
LinkedHashSet
TreeSet

## C Set data for 1m population

| Methods | ConcurrentSkipListSet J | ms | HashSet J | ms | LinkedHashSet J | ms | TreeSet J | ms |
|---|---|---|---|---|---|---|---|---|
| add | 14.0472 | 824 | 17.5243 | 1072 | 15.0643 | 876 | 14.1021 | 758 |
| addAll | 19.5092 | 1518 | 17.8589 | 1100 | 16.5155 | 983 | 13.5737 | 983 |
| clear | 11.5958 | 747 | 12.0199 | 764 | 12.2874 | 770 | 11.5565 | 758 |
| contains | 13.6576 | 870 | 16.6950 | 1014 | 15.6210 | 880 | 11.2337 | 682 |
| containsAll | 16.9809 | 1212 | 17.2110 | 1038 | 15.8865 | 886 | 12.3979 | 844 |
| iterateAll | 13.0184 | 785 | 18.1706 | 1091 | 15.4155 | 865 | 11.2088 | 684 |
| iterator | 13.2534 | 752 | 16.7433 | 1013 | 15.5284 | 850 | 11.0499 | 641 |
| remove | 12.7444 | 789 | 15.5699 | 949 | 13.6615 | 799 | 11.2653 | 675 |
| removeAll | 17.2849 | 1293 | 17.0514 | 998 | 14.5821 | 841 | 13.2071 | 937 |
| retainAll | 3621.9872 | 346898 | 3912.0129 | 384829 | 3584.3529 | 346337 | 4111.2397 | 408297 |
| toArray | 14.8120 | 875 | 17.8458 | 1070 | 14.3511 | 848 | 13.1271 | 750 |

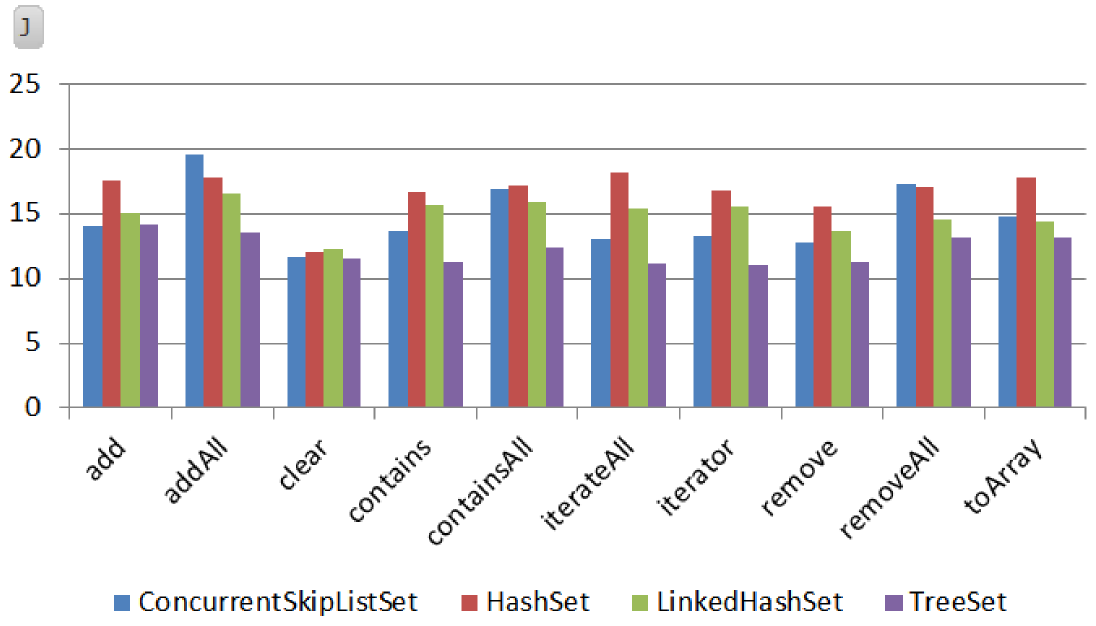

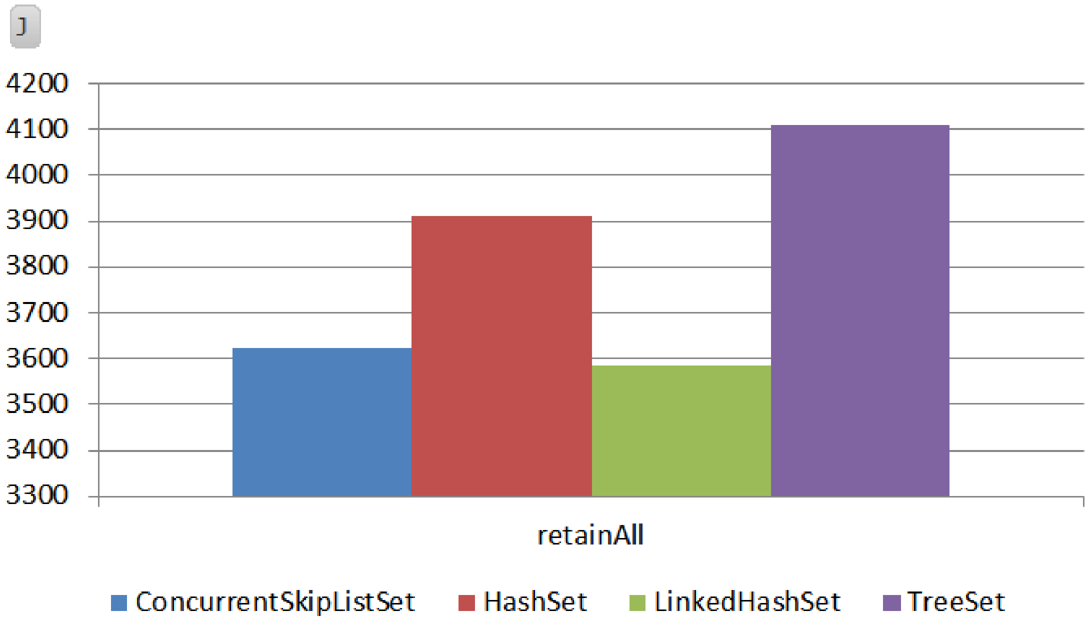

J
4200
4100
4000
3900
3800
3700
3600
3500
3400
3300
retainAll
ConcurrentSkipListSet
HashSet
LinkedHashSet
TreeSet

# D List data for 25k population

| Methods | ArrayList J | ArrayList ms | AttributeList J | AttributeList ms | CopyOn Write ArrayList J | CopyOn Write ArrayList ms | LinkedList J | LinkedList ms | RoleList J | RoleList ms | Role Unresolved List J | Role Unresolved List ms | Stack J | Stack ms | Vector J | Vector ms |
|---|---|---|---|---|---|---|---|---|---|---|---|---|---|---|---|---|
| add | 0.9773 | 71 | 1.1510 | 67 | 1.7839 | 117 | 1.8016 | 86 | 1.4801 | 76 | 1.1865 | 74 | 1.5659 | 76 | 1.5177 | 69 |
| addAll | 1.3353 | 76 | 1.0492 | 88 | 1.3586 | 82 | 1.1043 | 88 | 1.6661 | 76 | 1.8672 | 88 | 1.1015 | 88 | 1.7903 | 73 |
| addAlli | 1.7855 | 86 | 1.6035 | 68 | 1.1789 | 86 | 1.7272 | 99 | 1.5980 | 81 | 1.2497 | 85 | 1.2962 | 72 | 1.6268 | 90 |
| addI | 1.7125 | 93 | 1.3849 | 87 | 1.6558 | 119 | 1.6404 | 96 | 1.2718 | 85 | 1.3124 | 86 | 1.5287 | 83 | 1.4554 | 86 |
| clear | 1.1284 | 76 | 1.2409 | 75 | 1.7155 | 68 | 1.6497 | 74 | 1.6705 | 76 | 1.4304 | 80 | 1.6199 | 73 | 1.0574 | 71 |
| contains | 2.7568 | 166 | 2.4228 | 165 | 3.1768 | 167 | 3.1552 | 193 | 2.1751 | 162 | 2.4688 | 164 | 2.0128 | 166 | 2.1558 | 168 |
| containsAll | 1.5993 | 87 | 1.8053 | 92 | 2.1889 | 92 | 2.2887 | 118 | 1.3244 | 100 | 1.3930 | 96 | 1.2054 | 89 | 1.5091 | 87 |
| get | 2.0029 | 83 | 1.1171 | 78 | 1.4918 | 77 | 2.0168 | 109 | 2.2110 | 81 | 1.6613 | 71 | 1.8956 | 86 | 1.4978 | 73 |
| indexOf | 1.4447 | 76 | 2.0325 | 84 | 1.5682 | 70 | 2.6289 | 101 | 1.5674 | 79 | 1.1944 | 81 | 1.8090 | 81 | 2.0788 | 75 |
| iterateAll | 2.0701 | 79 | 1.0473 | 77 | 1.0103 | 73 | 2.6401 | 107 | 1.3605 | 85 | 1.7822 | 71 | 1.6036 | 81 | 1.1336 | 87 |
| iterator | 1.4893 | 84 | 1.1589 | 84 | 1.3922 | 72 | 1.7666 | 108 | 1.9760 | 73 | 1.3300 | 79 | 2.1895 | 84 | 1.6505 | 83 |
| lastIndexOf | 1.7750 | 99 | 1.7666 | 98 | 2.0383 | 94 | 2.5019 | 127 | 1.8914 | 92 | 1.4211 | 95 | 1.2260 | 84 | 1.2296 | 96 |
| listIterator | 1.4457 | 76 | 1.6190 | 84 | 1.3737 | 71 | 2.5003 | 106 | 1.3380 | 80 | 1.5176 | 85 | 1.6354 | 69 | 1.2746 | 81 |
| listIteratori | 1.7356 | 78 | 1.1552 | 81 | 1.5160 | 77 | 2.1996 | 105 | 1.7588 | 79 | 1.0334 | 80 | 1.8799 | 85 | 1.7545 | 78 |
| remove | 1.1308 | 96 | 1.4480 | 85 | 2.1946 | 162 | 1.6924 | 98 | 1.4560 | 84 | 1.1368 | 85 | 1.2663 | 96 | 1.4973 | 82 |
| removeAll | 8.0905 | 671 | 7.8108 | 697 | 7.3237 | 666 | 8.3150 | 752 | 7.6148 | 692 | 7.9911 | 664 | 7.3824 | 654 | 7.1281 | 665 |
| removei | 1.9135 | 85 | 1.3534 | 92 | 2.2858 | 118 | 1.7174 | 100 | 1.6308 | 85 | 1.6369 | 89 | 1.5850 | 81 | 1.5486 | 90 |
| retainAll | 2.7037 | 193 | 2.7845 | 200 | 2.6052 | 198 | 2.5982 | 205 | 3.0973 | 197 | 2.4172 | 200 | 2.7635 | 242 | 3.4019 | 245 |
| set | 0.9476 | 64 | 1.5943 | 70 | 1.9669 | 110 | 2.0474 | 112 | 1.5249 | 76 | 1.2312 | 73 | 1.4938 | 75 | 1.4957 | 72 |
| sublist | 1.3108 | 76 | 1.6021 | 80 | 1.4792 | 80 | 1.8457 | 98 | 1.4910 | 85 | 1.5117 | 71 | 1.7082 | 75 | 0.9414 | 75 |
| toArray | 1.6418 | 84 | 1.5024 | 84 | 2.0934 | 73 | 1.6739 | 106 | 1.5418 | 79 | 1.7455 | 83 | 1.5694 | 69 | 2.0213 | 80 |

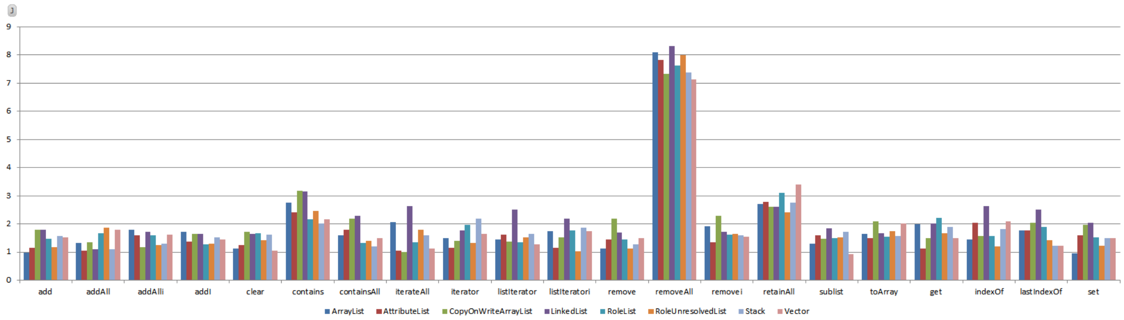

# E List data for 250k population

| Methods | ArrayList J | ArrayList ms | AttributeList J | AttributeList ms | CopyOn Write ArrayList J | CopyOn Write ArrayList ms | LinkedList J | LinkedList ms | RoleList J | RoleList ms | Role Unresolved List J | Role Unresolved List ms | Stack J | Stack ms | Vector J | Vector ms |
|---|---|---|---|---|---|---|---|---|---|---|---|---|---|---|---|---|
| add | 3.8352 | 225 | 4.6749 | 228 | 59.9706 | 5552 | 6.2024 | 294 | 4.0685 | 223 | 4.3435 | 222 | 4.3659 | 225 | 4.0186 | 221 |
| addAll | 4.0158 | 213 | 4.1970 | 213 | 3.7459 | 212 | 6.3524 | 306 | 4.0595 | 236 | 4.1118 | 233 | 4.0586 | 211 | 3.8572 | 217 |
| addAlli | 3.1822 | 200 | 3.6327 | 196 | 3.6868 | 195 | 6.5870 | 318 | 3.8740 | 221 | 4.3522 | 198 | 4.3606 | 222 | 3.9313 | 229 |
| addI | 17.9630 | 1366 | 17.5091 | 1372 | 64.4550 | 6091 | 13.8804 | 1037 | 17.3695 | 1371 | 17.1374 | 1366 | 17.4695 | 1365 | 17.4099 | 1368 |
| clear | 3.6320 | 218 | 4.2446 | 238 | 4.1154 | 219 | 4.2423 | 225 | 4.3240 | 221 | 4.0848 | 237 | 4.1995 | 220 | 4.4717 | 238 |
| contains | 149.2101 | 14930 | 143.8105 | 14297 | 138.7096 | 13608 | 177.4864 | 17145 | 143.5583 | 14361 | 144.8360 | 14440 | 148.3477 | 14941 | 147.6217 | 14919 |
| containsAll | 14.2118 | 1210 | 14.1992 | 1161 | 15.4383 | 1282 | 16.9662 | 1399 | 13.9955 | 1178 | 14.3545 | 1184 | 14.0874 | 1155 | 14.2835 | 1160 |
| get | 3.7491 | 225 | 3.8010 | 196 | 3.3272 | 196 | 9.1736 | 738 | 4.1234 | 194 | 3.3873 | 203 | 4.1009 | 200 | 3.4824 | 195 |
| indexOf | 4.2838 | 207 | 4.2417 | 208 | 4.0170 | 213 | 5.5329 | 275 | 4.1047 | 230 | 3.6321 | 201 | 3.6502 | 202 | 4.0763 | 204 |
| iterateAll | 3.9417 | 205 | 3.8646 | 206 | 4.1047 | 200 | 6.0103 | 303 | 3.9434 | 229 | 4.3596 | 209 | 3.9510 | 224 | 4.0285 | 232 |
| iterator | 4.2709 | 196 | 4.2472 | 194 | 3.7052 | 200 | 6.2585 | 266 | 3.7146 | 201 | 3.7738 | 204 | 3.4071 | 204 | 4.2383 | 204 |
| lastIndexOf | 27.2224 | 2438 | 26.7242 | 2408 | 26.5297 | 2448 | 36.6855 | 3260 | 26.6724 | 2413 | 26.8274 | 2388 | 26.2273 | 2409 | 26.5668 | 2413 |
| listIterator | 4.0923 | 199 | 3.8791 | 197 | 3.4499 | 201 | 4.7948 | 271 | 3.5211 | 198 | 3.5665 | 197 | 3.5485 | 195 | 3.8970 | 200 |
| listIteratori | 3.5178 | 197 | 4.8897 | 195 | 4.1712 | 197 | 5.6153 | 264 | 4.1498 | 195 | 3.7611 | 196 | 3.4433 | 200 | 3.8707 | 195 |
| remove | 16.7118 | 1293 | 16.0287 | 1296 | 85.5149 | 8048 | 5.2105 | 243 | 16.3957 | 1305 | 16.9656 | 1294 | 15.8466 | 1297 | 16.4117 | 1290 |
| removeAll | 800.6362 | 74570 | 815.9125 | 75055 | 848.7941 | 77949 | 829.8120 | 76059 | 812.6019 | 75188 | 803.4346 | 74341 | 811.8826 | 75083 | 816.0893 | 75628 |
| removei | 15.7604 | 1238 | 15.5615 | 1238 | 57.5978 | 5359 | 9.4499 | 731 | 15.3716 | 1232 | 15.9824 | 1235 | 15.9731 | 1225 | 15.4837 | 1243 |
| retainAll | 191.2629 | 17515 | 189.2622 | 17436 | 187.5156 | 17258 | 189.0232 | 17346 | 185.6256 | 17141 | 192.1342 | 17445 | 246.8980 | 22740 | 256.3624 | 23843 |
| set | 4.0179 | 204 | 3.8355 | 207 | 55.3024 | 5215 | 9.4216 | 757 | 3.9253 | 211 | 3.8588 | 210 | 4.1395 | 208 | 4.2365 | 236 |
| sublist | 4.1009 | 203 | 3.4186 | 202 | 3.5210 | 194 | 5.3223 | 272 | 3.6955 | 197 | 3.9814 | 196 | 3.7111 | 194 | 3.9882 | 198 |
| toArray | 3.6473 | 200 | 3.8151 | 202 | 3.5124 | 196 | 6.5844 | 273 | 3.8092 | 195 | 3.7162 | 196 | 3.7170 | 195 | 3.1472 | 195 |

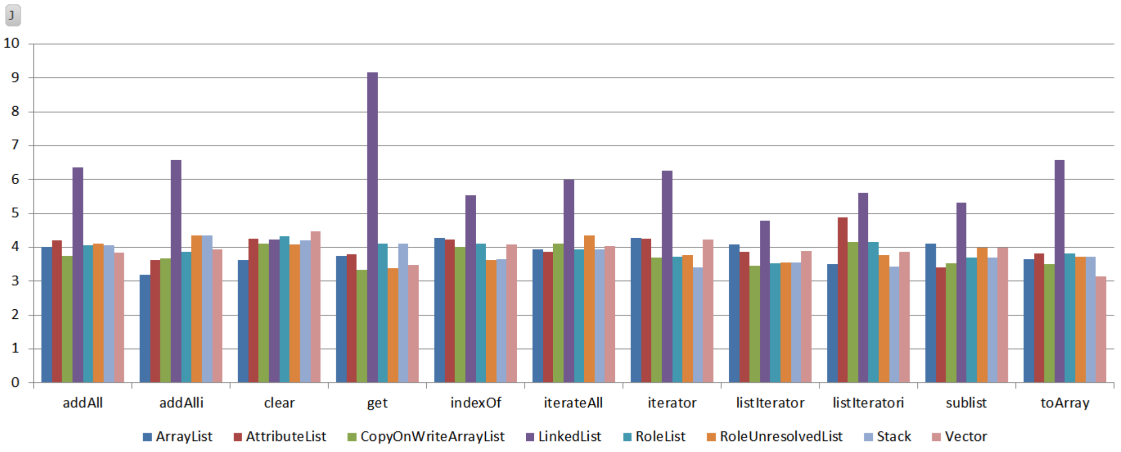

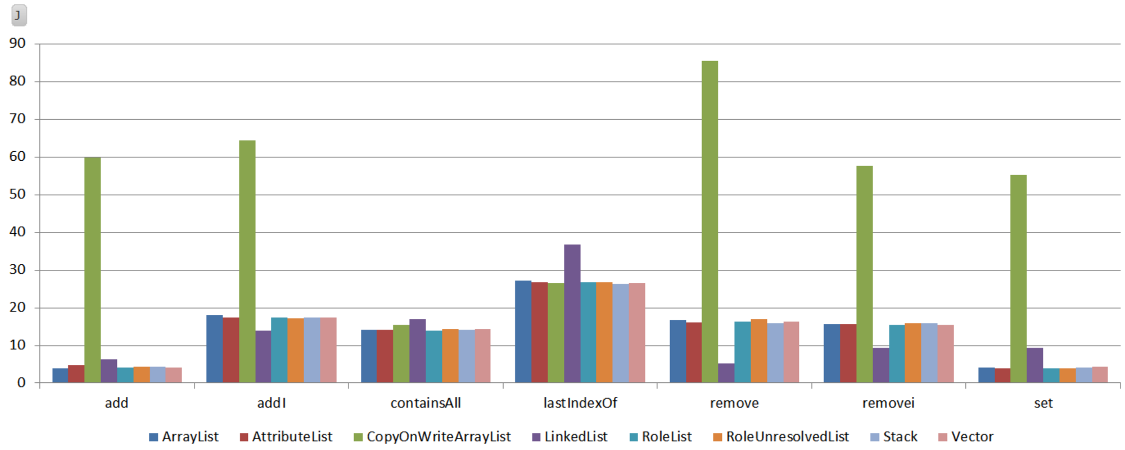

90
80
70
60
50
40
30
20
10
0
add
addI
containsAll
lastIndexOf
remove
removei
set
ArrayList
AttributeList
CopyOnWriteArrayList
LinkedList
RoleList
RoleUnresolvedList
Stack
Vector


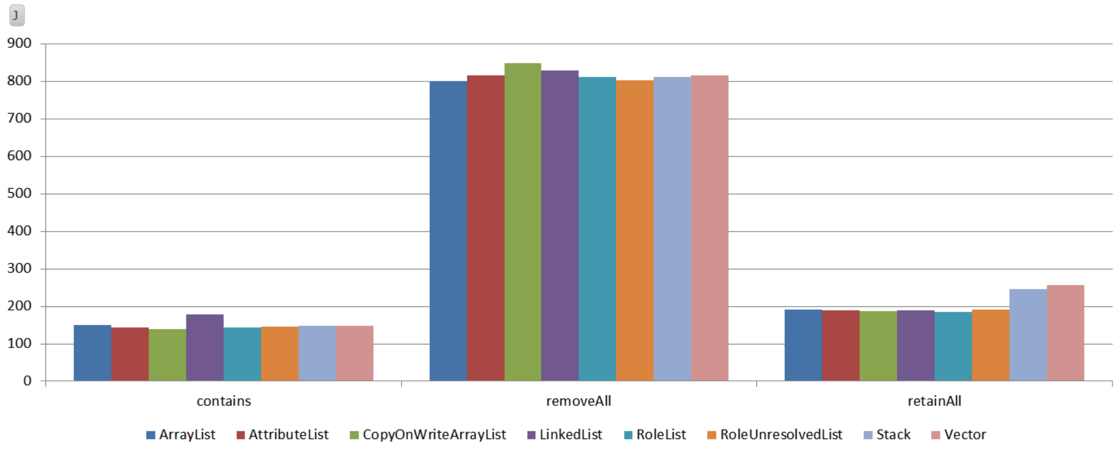

900
800
700
600
500
400
300
200
100
0
contains
removeAll
retainAll
ArrayList
AttributeList
CopyOnWriteArrayList
LinkedList
RoleList
RoleUnresolvedList
Stack
Vector

# F List data for 1m population

| Methods | ArrayList J | ArrayList ms | AttributeList J | AttributeList ms | CopyOn Write J | CopyOn Write ms | LinkedList J | LinkedList ms | RoleList J | RoleList ms | Role Unresolved J | Role Unresolved ms | Stack J | Stack ms | Vector J | Vector ms |
|---|---|---|---|---|---|---|---|---|---|---|---|---|---|---|---|---|
| add | 12.0464 | 701 | 12.7195 | 707 | 1192.1624 | 116076 | 13.1935 | 728 | 12.4607 | 709 | 12.3262 | 706 | 11.7879 | 722 | 11.3576 | 696 |
| addAll | 10.9094 | 648 | 11.3724 | 641 | 11.9216 | 660 | 14.2490 | 817 | 11.3734 | 637 | 11.4211 | 639 | 10.4004 | 642 | 10.7678 | 649 |
| addAlli | 10.1839 | 615 | 10.5913 | 622 | 10.5091 | 634 | 14.0827 | 834 | 10.4132 | 613 | 10.0168 | 611 | 10.0941 | 615 | 10.5229 | 617 |
| addI | 308.6728 | 28059 | 308.4402 | 28070 | 1347.1859 | 128466 | 190.3535 | 18902 | 312.4176 | 28542 | 313.0971 | 28577 | 312.1597 | 28570 | 312.8684 | 28688 |
| clear | 11.6159 | 740 | 11.7247 | 730 | 12.0538 | 732 | 12.0858 | 742 | 11.6814 | 738 | 11.7761 | 736 | 12.2983 | 736 | 11.7146 | 736 |
| contains | 1970.9064 | 195324 | 1952.7448 | 191984 | 1979.2615 | 195337 | 2466.3537 | 239826 | 1950.6017 | 191656 | 1959.7723 | 193343 | 1957.1560 | 192235 | 1968.4488 | 193401 |
| containsAll | 185.4605 | 17164 | 185.8306 | 17224 | 199.4027 | 18557 | 270.4051 | 24800 | 185.9840 | 17178 | 186.6167 | 17244 | 187.1497 | 17239 | 186.1992 | 17221 |
| get | 10.9069 | 616 | 11.4765 | 625 | 10.7958 | 629 | 81.1299 | 8346 | 11.3632 | 643 | 11.0016 | 626 | 10.9420 | 621 | 10.7961 | 616 |
| indexOf | 12.3355 | 752 | 12.5442 | 752 | 12.4852 | 751 | 13.0304 | 824 | 12.5427 | 758 | 11.8597 | 750 | 12.6218 | 771 | 12.1569 | 764 |
| iterateAll | 11.4806 | 659 | 11.3767 | 646 | 10.8094 | 646 | 12.0847 | 692 | 10.6485 | 640 | 11.0305 | 644 | 11.9679 | 741 | 11.3126 | 737 |
| iterator | 11.0537 | 635 | 10.9354 | 629 | 10.6816 | 624 | 11.9186 | 694 | 10.5633 | 633 | 10.0707 | 622 | 10.9189 | 653 | 11.3553 | 643 |
| lastIndexOf | 387.2730 | 36766 | 388.6052 | 37032 | 387.0817 | 37231 | 489.1250 | 46240 | 393.5686 | 37582 | 390.2053 | 37104 | 386.6704 | 37474 | 386.9537 | 37475 |
| listIterator | 10.6885 | 611 | 11.4602 | 631 | 11.4474 | 657 | 12.0396 | 669 | 11.3297 | 629 | 11.2530 | 630 | 11.3042 | 623 | 10.8957 | 615 |
| listIteratori | 11.5547 | 640 | 11.8432 | 618 | 10.8368 | 629 | 12.1197 | 741 | 11.1662 | 622 | 11.3287 | 643 | 10.8977 | 629 | 10.9616 | 611 |
| remove | 286.8151 | 25810 | 289.7602 | 26253 | 1382.3727 | 130720 | 11.2295 | 639 | 290.6235 | 26322 | 288.9534 | 26146 | 288.1555 | 25858 | 290.4005 | 26330 |
| removeAll | 6240.3017 | 616088 | 6254.3095 | 619221 | 7633.4344 | 756859 | 6031.4099 | 600757 | 6240.6818 | 616568 | 6242.6897 | 616035 | 7481.8537 | 741031 | 7491.7295 | 740725 |
| removei | 264.0750 | 23596 | 264.7749 | 23789 | 1193.7827 | 113704 | 80.0698 | 8312 | 267.6469 | 24018 | 263.0561 | 23579 | 266.6137 | 23979 | 265.2319 | 23828 |
| retainAll | 4165.0922 | 415147 | 4108.4192 | 409992 | 4285.7077 | 426197 | 4046.2904 | 402778 | 4125.8655 | 411737 | 4143.7322 | 413506 | 6116.5527 | 605233 | 6083.4340 | 606689 |
| set | 11.5278 | 653 | 10.7694 | 647 | 1107.5213 | 107726 | 81.0687 | 8381 | 11.5072 | 655 | 11.8232 | 642 | 11.4580 | 673 | 11.1637 | 656 |
| sublist | 10.9601 | 611 | 10.7711 | 636 | 11.1858 | 622 | 11.7203 | 676 | 10.9904 | 638 | 10.8467 | 634 | 11.3011 | 636 | 10.6396 | 627 |
| toArray | 10.7242 | 612 | 11.5362 | 642 | 10.4389 | 628 | 14.5166 | 796 | 10.6314 | 623 | 10.6248 | 619 | 10.6683 | 614 | 11.0372 | 637 |

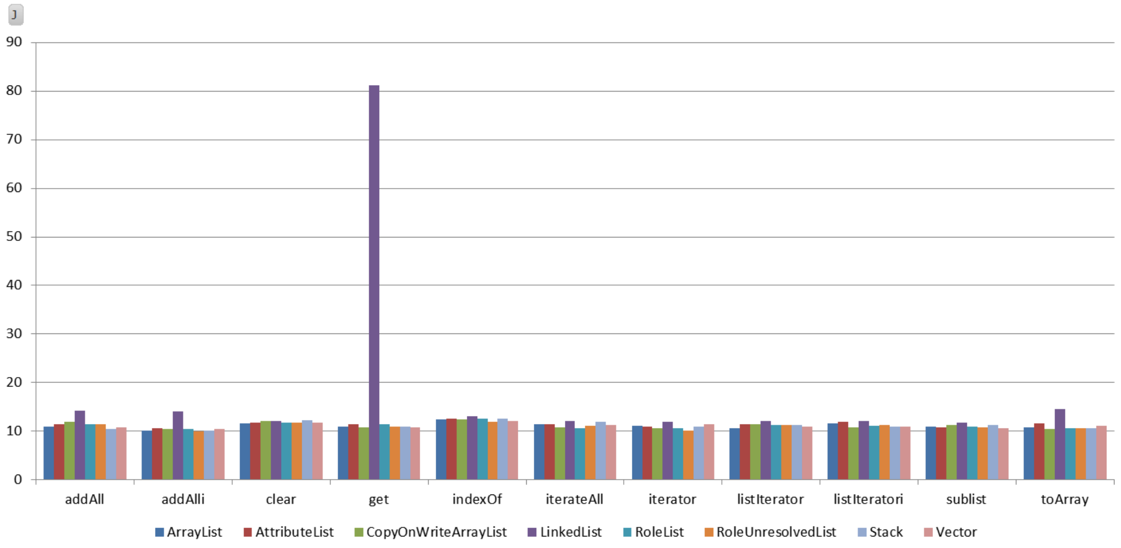

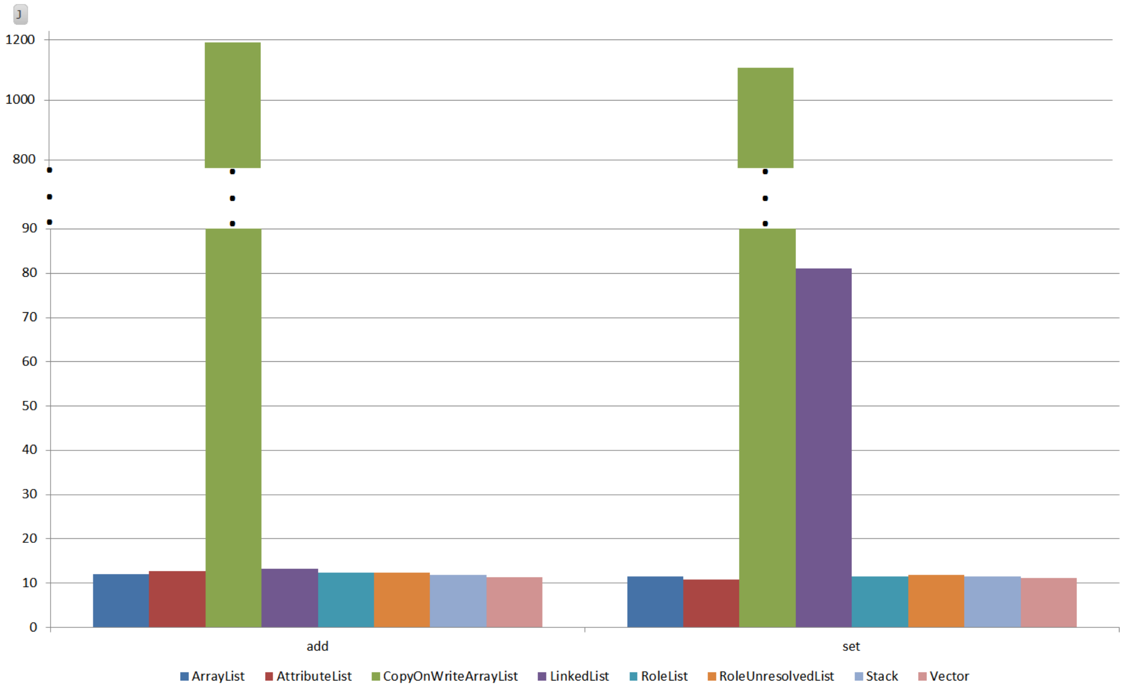

J
1200
1000
800
90
80
70
60
50
40
30
20
10
0
add
set
ArrayList
AttributeList
CopyOnWriteArrayList
LinkedList
RoleList
RoleUnresolvedList
Stack
Vector


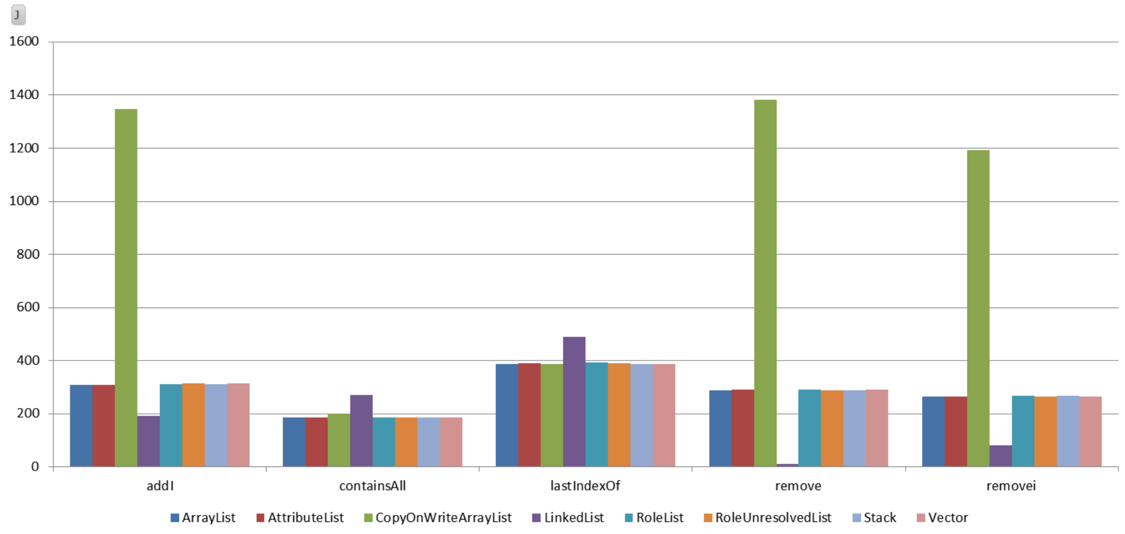

J
1600
1400
1200
1000
800
600
400
200
0
addI
containsAll
lastIndexOf
remove
removei
ArrayList
AttributeList
CopyOnWriteArrayList
LinkedList
RoleList
RoleUnresolvedList
Stack
Vector

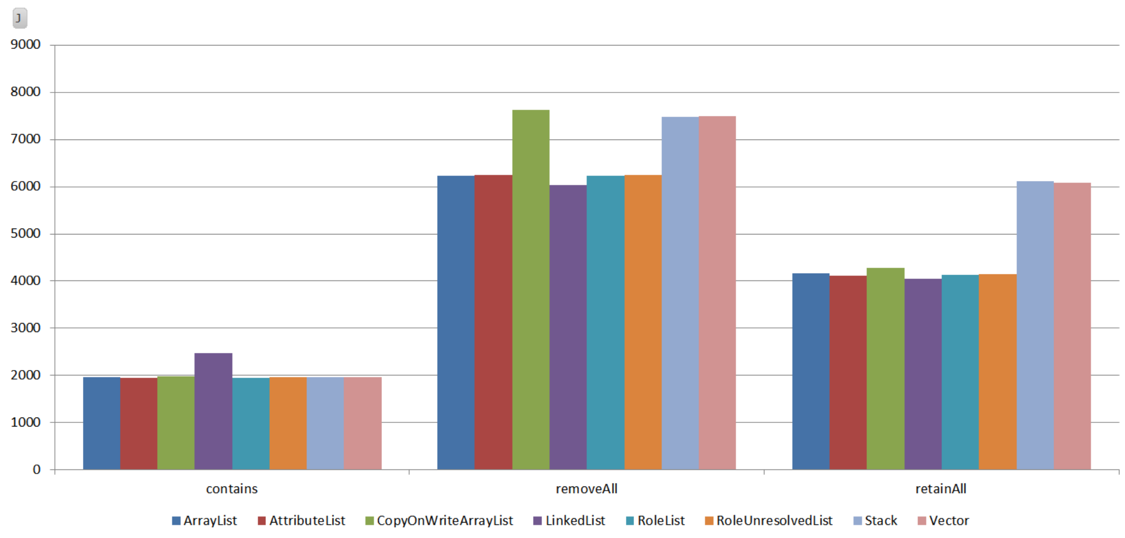
9000
8000
7000
6000
5000
4000
3000
2000
1000
0
contains
removeAll
retainAll
ArrayList
AttributeList
CopyOnWriteArrayList
LinkedList
RoleList
RoleUnresolvedList
Stack
Vector

# G Map data for 25k population

| Methods | ConcurrentHashMap J | ms | ConcurrentSkipListMap J | ms | HashMap J | ms | Hashtable J | ms | LinkedHashMap J | ms | Properties J | ms | SimpleBindings J | ms | TreeMap J | ms | UIDefaults J | ms | WeakHashMap J | ms |
|---|---|---|---|---|---|---|---|---|---|---|---|---|---|---|---|---|---|---|---|---|
| clear | 2.0276 | 94 | 2.2961 | 88 | 1.8395 | 104 | 1.5761 | 94 | 1.5025 | 97 | 2.0777 | 98 | 2.1401 | 106 | 1.6706 | 98 | 1.8143 | 105 | 1.9941 | 95 |
| containsKey | 2.3132 | 105 | 2.1693 | 123 | 2.1343 | 103 | 1.8582 | 94 | 1.8726 | 103 | 1.6018 | 107 | 1.8055 | 99 | 1.9452 | 100 | 2.3366 | 89 | 1.9675 | 108 |
| containsValue | 21.5611 | 2305 | 7.8032 | 643 | 8.3615 | 683 | 8.4957 | 765 | 6.1326 | 462 | 7.3755 | 692 | 7.9912 | 678 | 9.1771 | 847 | 7.9341 | 714 | 6.7072 | 562 |
| entrySet | 2.2878 | 93 | 2.2363 | 116 | 1.8531 | 108 | 2.1332 | 107 | 1.8362 | 113 | 1.7800 | 97 | 2.1557 | 102 | 2.1617 | 115 | 1.7087 | 105 | 1.4666 | 102 |
| get | 2.3106 | 103 | 1.9972 | 119 | 1.8120 | 102 | 1.4071 | 100 | 1.8252 | 116 | 1.7851 | 97 | 1.5359 | 100 | 2.2331 | 115 | 1.5252 | 89 | 1.7185 | 103 |
| iterateAll | 2.1041 | 96 | 1.8353 | 115 | 2.6673 | 100 | 1.5343 | 91 | 1.6462 | 111 | 1.6362 | 100 | 2.0472 | 116 | 1.9122 | 111 | 1.6574 | 95 | 1.7139 | 106 |
| keySet | 1.7287 | 95 | 2.4889 | 124 | 1.6813 | 114 | 2.2226 | 99 | 1.8328 | 103 | 1.4866 | 92 | 2.0630 | 106 | 2.1680 | 110 | 1.5547 | 99 | 1.8749 | 105 |
| put | 1.8591 | 104 | 2.2888 | 102 | 2.4628 | 92 | 1.3123 | 96 | 2.0338 | 108 | 1.7038 | 107 | 2.1646 | 102 | 1.4355 | 91 | 2.1204 | 93 | 2.5784 | 105 |
| putAll | 1.4147 | 95 | 2.2852 | 122 | 1.7564 | 100 | 1.5949 | 105 | 1.8608 | 113 | 1.3097 | 95 | 2.1461 | 112 | 1.8914 | 116 | 2.3094 | 87 | 2.0750 | 108 |
| remove | 1.8574 | 92 | 2.2131 | 105 | 1.9256 | 109 | 1.6067 | 97 | 2.2300 | 106 | 1.9660 | 98 | 2.2178 | 106 | 1.8133 | 101 | 1.6888 | 92 | 2.4103 | 103 |
| values | 1.8279 | 85 | 2.4690 | 116 | 2.5755 | 109 | 2.2266 | 94 | 2.0009 | 107 | 1.9120 | 111 | 2.0692 | 108 | 1.4467 | 105 | 1.6533 | 100 | 2.4628 | 111 |

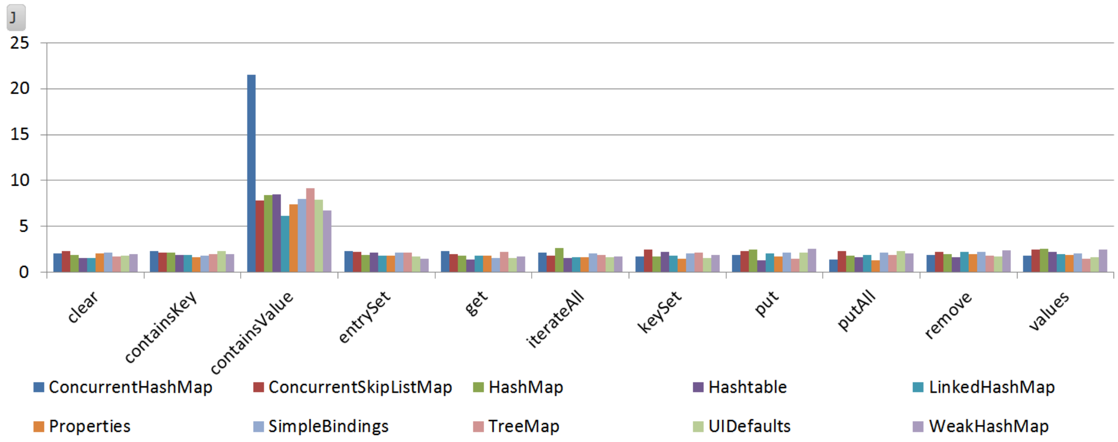

# H Map data for 250k population

| Methods | ConcurrentHashMap | | ConcurrentSkipListMap | | HashMap | | Hashtable | | LinkedHashMap | |
|---|---|---|---|---|---|---|---|---|---|---|
| | J | ms | J | ms | J | ms | J | ms | J | ms |
| clear | 8.0929 | 532 | 8.6506 | 548 | 8.2128 | 526 | 8.4732 | 522 | 7.9924 | 518 |
| containsKey | 7.8434 | 426 | 9.1539 | 473 | 9.1804 | 550 | 7.8745 | 451 | 7.8521 | 429 |
| containsValue | 3911.4124 | 461730 | 1334.8256 | 154701 | 730.9166 | 75444 | 1128.1868 | 127397 | 545.2480 | 55788 |
| entrySet | 8.0325 | 434 | 8.0541 | 466 | 9.0436 | 547 | 7.8135 | 438 | 7.8607 | 441 |
| get | 7.4986 | 434 | 8.1773 | 465 | 9.4016 | 546 | 8.2263 | 449 | 8.0936 | 419 |
| iterateAll | 7.5645 | 487 | 8.3979 | 494 | 9.2449 | 570 | 8.9272 | 477 | 7.8789 | 451 |
| keySet | 7.3338 | 436 | 8.2838 | 456 | 9.4461 | 570 | 8.0567 | 448 | 7.5861 | 433 |
| put | 8.0530 | 458 | 8.6610 | 467 | 9.5894 | 576 | 8.4029 | 452 | 8.3766 | 432 |
| putAll | 7.9165 | 460 | 9.6607 | 566 | 9.6678 | 562 | 7.4861 | 443 | 7.6870 | 421 |
| remove | 8.8059 | 455 | 8.0675 | 474 | 9.1076 | 545 | 7.9131 | 437 | 8.4532 | 422 |
| values | 7.3602 | 440 | 8.7056 | 463 | 9.4056 | 571 | 7.9879 | 450 | 7.8246 | 438 |

| Methods | Properties | | Simple Bindings | | TreeMap | | UIDefaults | | WeakHashMap | |
|---|---|---|---|---|---|---|---|---|---|---|
| | J | ms | J | ms | J | ms | J | ms | J | ms |
| clear | 8.0495 | 529 | 8.4215 | 516 | 8.5468 | 543 | 8.4711 | 527 | 8.1116 | 522 |
| containsKey | 8.0387 | 451 | 9.1259 | 536 | 7.1873 | 415 | 7.9168 | 452 | 10.8584 | 610 |
| containsValue | 1166.8370 | 131071 | 745.1696 | 76840 | 1606.2652 | 183898 | 1204.5573 | 136323 | 912.0360 | 91357 |
| entrySet | 7.7498 | 442 | 8.6253 | 540 | 7.3000 | 399 | 8.7348 | 440 | 10.3130 | 621 |
| get | 8.1691 | 453 | 9.3113 | 542 | 7.2236 | 415 | 8.8114 | 442 | 10.4985 | 621 |
| iterateAll | 8.5419 | 477 | 9.7741 | 562 | 7.3954 | 452 | 8.5096 | 475 | 10.4295 | 630 |
| keySet | 8.0351 | 452 | 9.3002 | 533 | 7.5795 | 415 | 7.8576 | 455 | 9.9974 | 614 |
| put | 8.3302 | 448 | 9.6672 | 557 | 8.2926 | 421 | 7.9345 | 450 | 11.2110 | 633 |
| putAll | 7.6266 | 441 | 9.3364 | 550 | 7.5239 | 470 | 7.9134 | 451 | 9.7825 | 626 |
| remove | 8.1008 | 443 | 8.3784 | 531 | 8.0151 | 437 | 7.7442 | 447 | 8.4500 | 533 |
| values | 8.4208 | 441 | 8.9347 | 548 | 7.3330 | 415 | 8.4531 | 451 | 10.5991 | 615 |

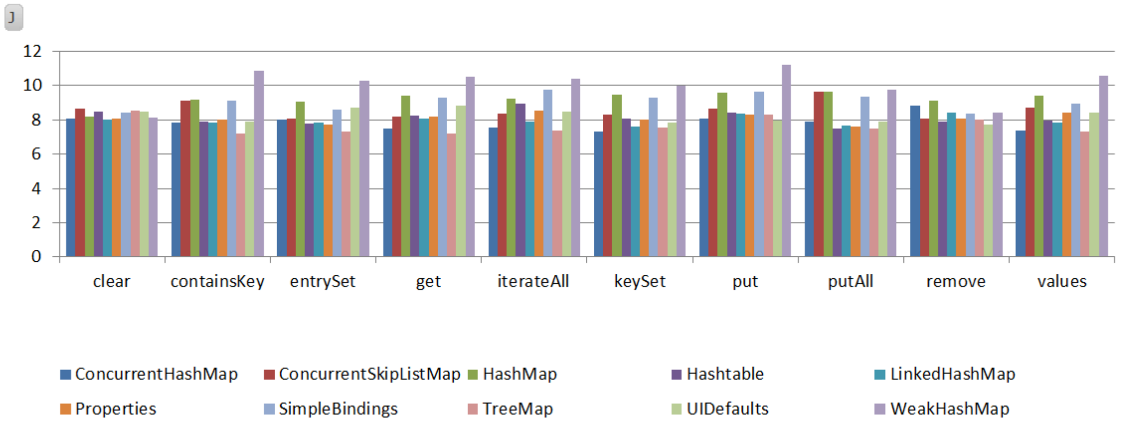


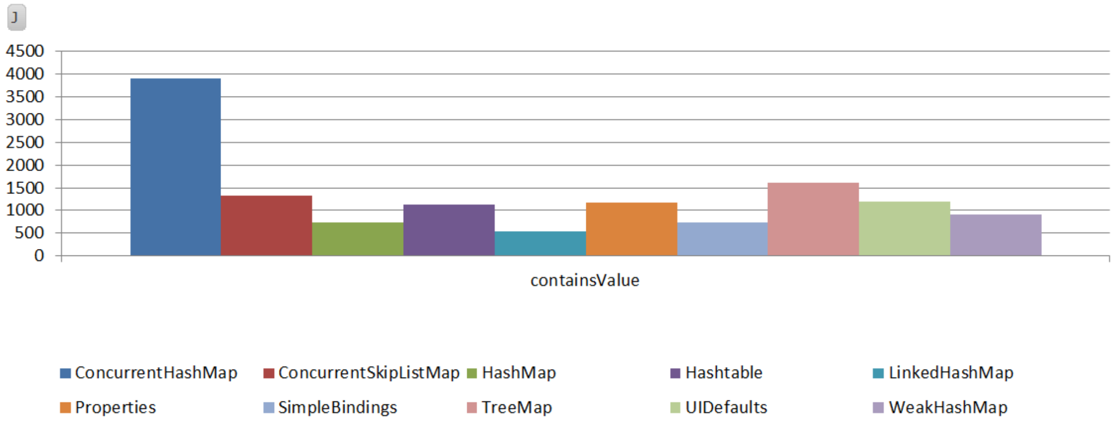

# I Map data for 1m population

| Methods | Concurrent HashMap J | ms | Concurrent SkipList Map J | ms | HashMap J | ms | Hashtable J | ms | Linked HashMap J | ms |
|---|---|---|---|---|---|---|---|---|---|---|
| clear | 32.1468 | 2086 | 31.6883 | 2020 | 31.6585 | 1997 | 31.4659 | 2009 | 31.7548 | 2002 |
| containsKey | 25.3230 | 1645 | 27.0269 | 1707 | 33.4752 | 2056 | 27.0329 | 1615 | 26.1077 | 1585 |
| containsValue | 5110.1689 | 602187 | 5223.6619 | 602035 | 5809.9971 | 602007 | 5377.3805 | 602040 | 5719.4071 | 602019 |
| entrySet | 26.2053 | 1631 | 26.3433 | 1630 | 34.2838 | 2108 | 27.4266 | 1637 | 27.3013 | 1625 |
| get | 25.4475 | 1658 | 26.8225 | 1668 | 33.0373 | 2060 | 26.7896 | 1603 | 27.0924 | 1605 |
| iterateAll | 29.0126 | 1931 | 26.4318 | 1701 | 34.3681 | 2158 | 27.3898 | 1701 | 27.3926 | 1655 |
| keySet | 26.4697 | 1654 | 26.1301 | 1613 | 33.2621 | 2041 | 27.0295 | 1634 | 27.3374 | 1638 |
| put | 27.0194 | 1759 | 28.0145 | 1745 | 34.9660 | 2168 | 28.3543 | 1712 | 26.1753 | 1552 |
| putAll | 26.5031 | 1764 | 29.3885 | 2020 | 35.0481 | 2174 | 28.0358 | 1704 | 26.2283 | 1580 |
| remove | 25.5665 | 1667 | 26.6545 | 1694 | 32.3202 | 1973 | 26.4978 | 1591 | 25.9951 | 1581 |
| values | 26.3867 | 1663 | 26.6376 | 1632 | 32.8656 | 2033 | 26.9196 | 1630 | 28.2103 | 1628 |

| Methods | Properties J | ms | Simple Bindings J | ms | TreeMap J | ms | UIDefaults J | ms | Weak HashMap J | ms |
|---|---|---|---|---|---|---|---|---|---|---|
| clear | 31.6198 | 2018 | 31.3525 | 1978 | 32.2024 | 2015 | 31.6685 | 2018 | 31.7730 | 1992 |
| containsKey | 26.8887 | 1634 | 32.9557 | 2026 | 24.2985 | 1539 | 26.4794 | 1615 | 38.1398 | 2362 |
| containsValue | 5408.3341 | 602026 | 5781.2350 | 602023 | 5291.3279 | 602031 | 5454.6906 | 602028 | 5931.2509 | 602055 |
| entrySet | 27.1060 | 1621 | 32.9119 | 2043 | 23.8757 | 1478 | 26.7149 | 1624 | 38.6346 | 2417 |
| get | 28.3008 | 1683 | 33.4063 | 2061 | 25.0432 | 1545 | 26.9511 | 1601 | 38.2429 | 2357 |
| iterateAll | 27.9918 | 1717 | 33.7128 | 2100 | 24.8704 | 1627 | 28.1027 | 1702 | 34.2753 | 2250 |
| keySet | 26.3382 | 1621 | 33.7798 | 2055 | 24.1255 | 1502 | 27.0168 | 1618 | 38.2719 | 2376 |
| put | 28.0086 | 1731 | 34.3807 | 2141 | 25.3354 | 1587 | 28.5027 | 1712 | 36.0024 | 2211 |
| putAll | 27.5977 | 1682 | 34.2556 | 2121 | 26.6613 | 1725 | 27.4983 | 1673 | 38.2742 | 2380 |
| remove | 26.2373 | 1598 | 31.6204 | 1937 | 24.4253 | 1530 | 27.1669 | 1612 | 35.4727 | 2158 |
| values | 26.8990 | 1621 | 33.3910 | 2052 | 24.2967 | 1477 | 26.7752 | 1639 | 38.9120 | 2413 |

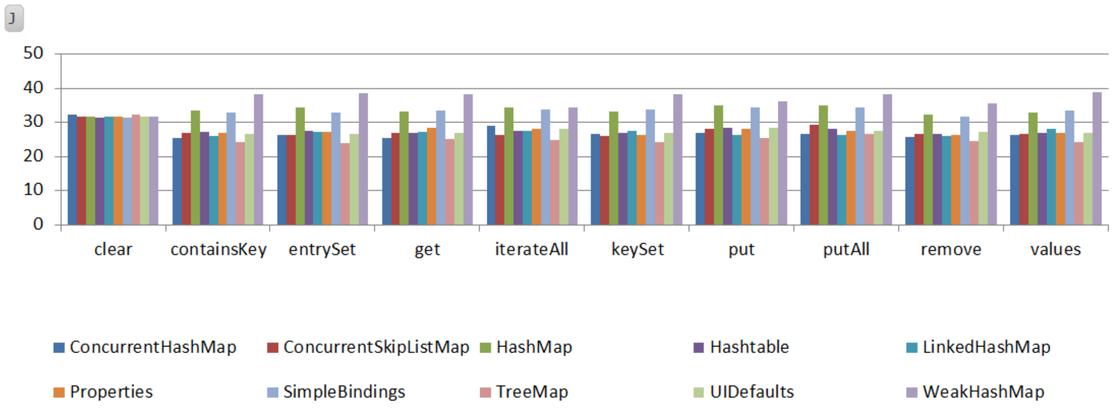


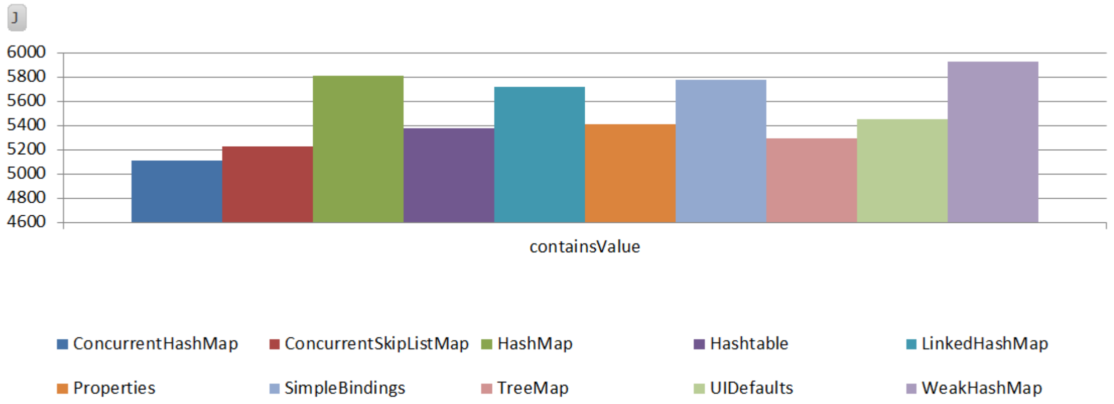

Supplement: Supplementary file 1 [file appendixGreens.pdf]
